# Supplementary material for: Spherical dust collapse in bimetric relativity: Bimetric polytropes
Source: arXiv:1904.08617 ancillary file (2019-04-18)
Supplement: Supplementary file 1 [file EoM.pdf]

# Bimetric polytropes, the regularized equations

Mikica Kocic

Created 2018-02-08, Last modified 2018-09-16

This notebook displays the equations used for the simulations.

## Definitions

```
SetDirectory@NotebookDirectory[];
```

```
$debugMode = False;
```

```
Get["bimetric-ss-solver.m"]
```

```
dump[eqs_] := (Print@PrintNice@Row@{#[[1]], " = ", #[[2]]} & /@ eqs[[All, {2, 3}]]);
```

## The evolution equations for g

```
EoM$gEvol // dump
```

$$\partial_t A = -\frac{\partial_r p p^2 \alpha}{\lambda^3} + A (\partial_r q + q D_A) + \frac{p \alpha D_\alpha}{\lambda} + \alpha \left( \frac{\partial_r p}{\lambda} + \frac{1}{3} A (-K - 2 K_\Delta) \right)$$

$$\partial_t B = \frac{B q + \frac{B p \alpha}{A \lambda}}{r} + B q D_B + \frac{B p \alpha D_B}{A \lambda} + \frac{1}{3} B \alpha (-K + K_\Delta)$$

$$\partial_t K_1 = \frac{1}{3} (\partial_r K + 2 \partial_r K_\Delta) q + \frac{(\partial_r K + 2 \partial_r K_\Delta) p \alpha}{3 A \lambda} + \frac{2 \alpha (D_A - 2 D_B)}{r A^2} + \alpha \left( \frac{-2 \partial_r D_B - \partial_r D_\alpha - 2 D_B^2 - D_\alpha^2 + D_A (2 D_B + D_\alpha)}{A^2} + \frac{1}{3} K (K + 2 K_\Delta) \right) + \left( -\frac{gJK}{3} - \frac{2 gJK_\Delta}{3} \right) \kappa_g$$

$$\partial_t K_2 = \frac{1}{3} (\partial_r K - \partial_r K_\Delta) q + \frac{(\partial_r K - \partial_r K_\Delta) p \alpha}{3 A \lambda} + \frac{\alpha \left( \frac{\sigma}{A B} + \frac{\sigma + D_A - 4 D_B - D_\alpha}{A^2} \right)}{r} + \alpha \left( \frac{-\partial_r D_B + D_A D_B - 2 D_B^2 - D_B D_\alpha}{A^2} + \frac{1}{3} K (K - K_\Delta) \right) + \left( -\frac{gJK}{3} + \frac{gJK_\Delta}{3} \right) \kappa_g$$

$$\partial_t D_A = \partial_{rr} q + \partial_r D_A q + \partial_r q D_A + \alpha \left( \frac{\frac{\partial_{rr} p - \partial_r p (D_A - 2 D_\alpha)}{\lambda^3}}{A} + p \left( -\frac{3 (\partial_r p)^2}{\lambda^5} + \frac{\partial_r D_\alpha - D_A D_\alpha + D_\alpha^2}{\lambda} \right) \right) + \frac{1}{3} (-\partial_r K - 2 \partial_r K_\Delta - D_\alpha (K + 2 K_\Delta))$$

$$\partial_t D_B = \partial_r \frac{q}{r} + \partial_r D_B q - \frac{p^3 \alpha}{r^2 A \lambda^3} + \partial_r q D_B + \frac{p \alpha (-D_A + D_\alpha)}{r A \lambda} + \frac{p \alpha (\partial_r D_B - D_A D_B + D_B D_\alpha)}{A \lambda} + \alpha \left( \frac{\partial_r \frac{p}{r} + \partial_r p D_B}{A \lambda^3} + \frac{1}{3} (-\partial_r K + \partial_r K_\Delta + D_\alpha (-K + K_\Delta)) \right)$$

$$\partial_t K = \partial_r K q + \frac{\partial_r K p \alpha}{A \lambda} + \frac{\alpha \left( \frac{2 \sigma}{A B} + \frac{2 (\sigma + 2 D_A - 6 D_B - D_\alpha)}{A^2} \right)}{r} + \alpha \left( K^2 + \frac{-4 \partial_r D_B - \partial_r D_\alpha - 6 D_B^2 - 2 D_B D_\alpha - D_\alpha^2 + D_A (4 D_B + D_\alpha)}{A^2} \right) - gJK \kappa_g$$

$$\partial_t K_\Delta = \partial_r K_\Delta q + \frac{\partial_r K_\Delta p \alpha}{A \lambda} + \frac{\alpha \left( -\frac{\sigma}{A B} + \frac{-\sigma + D_A + D_\alpha}{A^2} \right)}{r} + \alpha \left( \frac{-\partial_r D_B - \partial_r D_\alpha + D_B D_\alpha - D_\alpha^2 + D_A (D_B + D_\alpha)}{A^2} + K K_\Delta \right) - gJK_\Delta \kappa_g$$

$$\partial_t \sigma = \frac{\partial_r \frac{q}{r} A}{B} - \frac{p^3 \alpha}{r^2 B \lambda^3} + \frac{\frac{A q (D_A - D_B)}{B} + \frac{p \alpha (-D_B + D_\alpha)}{B \lambda}}{r} + \alpha \left( \frac{\partial_r \frac{p}{r}}{B \lambda^3} + \frac{A (-\partial_r K + \partial_r K_\Delta + 3 D_B K_\Delta)}{3 B} \right) + \frac{\langle R \rangle_1^2 A p \alpha \tilde{A} \kappa_g}{2 B} - \frac{\alpha \kappa_g \hat{S}_r}{2 B^3}$$

## The evolution equations for $f$

EoM\$fEvol // dump

$$\partial_t \tilde{A} = \frac{\partial_r \mathbf{p} \mathbf{p}^2 \tilde{\alpha}}{\lambda^3} + \tilde{A} \left( \partial_r \mathbf{q} + \mathbf{q} \tilde{D}_A \right) - \frac{\mathbf{p} \tilde{\alpha} \tilde{D}_\alpha}{\lambda} + \tilde{\alpha} \left( -\frac{\partial_r \mathbf{p}}{\lambda} + \frac{1}{3} \tilde{A} \left( -\tilde{K} - 2 \tilde{K}_\Delta \right) \right)$$

$$\partial_t \tilde{B} = \frac{\mathbf{q} \tilde{B} - \frac{\mathbf{p} \tilde{B} \tilde{\alpha}}{\lambda \tilde{A}}}{r} + \mathbf{q} \tilde{B} \tilde{D}_B - \frac{\mathbf{p} \tilde{B} \tilde{\alpha} \tilde{D}_B}{\lambda \tilde{A}} + \frac{1}{3} \tilde{B} \tilde{\alpha} \left( -\tilde{K} + \tilde{K}_\Delta \right)$$

$$\partial_t \tilde{K}_1 = \frac{1}{3} \left( \partial_r \tilde{K} + 2 \partial_r \tilde{K}_\Delta \right) \mathbf{q} - \frac{\left( \partial_r \tilde{K} + 2 \partial_r \tilde{K}_\Delta \right) \mathbf{p} \tilde{\alpha}}{3 \lambda \tilde{A}} + \left( -\frac{\boxed{fJK}}{3} - \frac{2 \boxed{fJK_\Delta}}{3} \right) \kappa_f +$$

$$\frac{2 \tilde{\alpha} \left( \tilde{D}_A - 2 \tilde{D}_B \right)}{r \tilde{A}^2} + \tilde{\alpha} \left( \frac{-2 \partial_r \tilde{D}_B - \partial_r \tilde{D}_\alpha - 2 \tilde{D}_B^2 - \tilde{D}_\alpha^2 + \tilde{D}_A \left( 2 \tilde{D}_B + \tilde{D}_\alpha \right)}{\tilde{A}^2} + \frac{1}{3} \tilde{K} \left( \tilde{K} + 2 \tilde{K}_\Delta \right) \right)$$

$$\partial_t \tilde{K}_2 = \frac{1}{3} \left( \partial_r \tilde{K} - \partial_r \tilde{K}_\Delta \right) \mathbf{q} + \frac{\left( -\partial_r \tilde{K} + \partial_r \tilde{K}_\Delta \right) \mathbf{p} \tilde{\alpha}}{3 \lambda \tilde{A}} + \left( -\frac{\boxed{fJK}}{3} + \frac{\boxed{fJK_\Delta}}{3} \right) \kappa_f +$$

$$\frac{\tilde{\alpha} \left( \frac{\tilde{\sigma}}{\tilde{A} \tilde{B}} + \frac{\tilde{\sigma} + \tilde{D}_A - 4 \tilde{D}_B - \tilde{D}_\alpha}{\tilde{A}^2} \right)}{r} + \tilde{\alpha} \left( \frac{-\partial_r \tilde{D}_B + \tilde{D}_A \tilde{D}_B - 2 \tilde{D}_B^2 - \tilde{D}_B \tilde{D}_\alpha}{\tilde{A}^2} + \frac{1}{3} \tilde{K} \left( \tilde{K} - \tilde{K}_\Delta \right) \right)$$

$$\partial_t \tilde{D}_A = \partial_{rr} \mathbf{q} + \partial_r \tilde{D}_A \mathbf{q} + \partial_r \mathbf{q} \tilde{D}_A + \frac{\tilde{\alpha} \left( -\partial_{rr} \mathbf{p} + \partial_r \mathbf{p} \left( \tilde{D}_A - 2 \tilde{D}_\alpha \right) \right)}{\lambda^3 \tilde{A}} +$$

$$\mathbf{p} \left( \frac{3 \left( \partial_r \mathbf{p} \right)^2 \tilde{\alpha}}{\lambda^5 \tilde{A}} + \frac{\tilde{\alpha} \left( -\partial_r \tilde{D}_\alpha + \left( \tilde{D}_A - \tilde{D}_\alpha \right) \tilde{D}_\alpha \right)}{\lambda \tilde{A}} \right) - \frac{1}{3} \tilde{\alpha} \left( \partial_r \tilde{K} + 2 \partial_r \tilde{K}_\Delta + \tilde{D}_\alpha \left( \tilde{K} + 2 \tilde{K}_\Delta \right) \right)$$

$$\partial_t \tilde{D}_B = \partial_r \frac{\mathbf{q}}{r} + \partial_r \tilde{D}_B \mathbf{q} + \frac{\mathbf{p}^3 \tilde{\alpha}}{r^2 \lambda^3 \tilde{A}} + \partial_r \mathbf{q} \tilde{D}_B + \frac{\mathbf{p} \tilde{\alpha} \left( \tilde{D}_A - \tilde{D}_\alpha \right)}{r \lambda \tilde{A}} -$$

$$\frac{\mathbf{p} \tilde{\alpha} \left( \partial_r \tilde{D}_B - \tilde{D}_A \tilde{D}_B + \tilde{D}_B \tilde{D}_\alpha \right)}{\lambda \tilde{A}} + \tilde{\alpha} \left( -\frac{\partial_r \frac{\mathbf{p}}{r} + \partial_r \mathbf{p} \tilde{D}_B}{\lambda^3 \tilde{A}} + \frac{1}{3} \left( -\partial_r \tilde{K} + \partial_r \tilde{K}_\Delta + \tilde{D}_\alpha \left( -\tilde{K} + \tilde{K}_\Delta \right) \right) \right)$$

$$\partial_t \tilde{K} = \partial_r \tilde{K} \mathbf{q} - \frac{\partial_r \tilde{K} \mathbf{p} \tilde{\alpha}}{\lambda \tilde{A}} - \boxed{fJK} \kappa_f + \frac{\tilde{\alpha} \left( \frac{2 \tilde{\sigma}}{\tilde{A} \tilde{B}} + \frac{2 \left( \tilde{\sigma} + 2 \tilde{D}_A - 6 \tilde{D}_B - \tilde{D}_\alpha \right)}{\tilde{A}^2} \right)}{r} +$$

$$\tilde{\alpha} \left( \tilde{K}^2 + \frac{1}{\tilde{A}^2} \left( -4 \partial_r \tilde{D}_B - \partial_r \tilde{D}_\alpha - 6 \tilde{D}_B^2 - 2 \tilde{D}_B \tilde{D}_\alpha - \tilde{D}_\alpha^2 + \tilde{D}_A \left( 4 \tilde{D}_B + \tilde{D}_\alpha \right) \right) \right)$$

$$\partial_t \tilde{K}_\Delta = \partial_r \tilde{K}_\Delta \mathbf{q} - \frac{\partial_r \tilde{K}_\Delta \mathbf{p} \tilde{\alpha}}{\lambda \tilde{A}} - \boxed{fJK_\Delta} \kappa_f + \frac{\tilde{\alpha} \left( -\frac{\tilde{\sigma}}{\tilde{A} \tilde{B}} + \frac{-\tilde{\sigma} + \tilde{D}_A + \tilde{D}_\alpha}{\tilde{A}^2} \right)}{r} + \tilde{\alpha} \left( \frac{-\partial_r \tilde{D}_B - \partial_r \tilde{D}_\alpha + \tilde{D}_B \tilde{D}_\alpha - \tilde{D}_\alpha^2 + \tilde{D}_A \left( \tilde{D}_B + \tilde{D}_\alpha \right)}{\tilde{A}^2} + \tilde{K} \tilde{K}_\Delta \right)$$

$$\partial_t \tilde{\sigma} = \frac{\partial_r \frac{\mathbf{q}}{r} \tilde{A}}{\tilde{B}} + \frac{\mathbf{p}^3 \tilde{\alpha}}{r^2 \lambda^3 \tilde{B}} - \frac{\langle \mathbf{R} \rangle_1^2 \mathbf{A} \mathbf{p} \tilde{A} \tilde{\alpha} \kappa_f}{2 \mathbf{R}^2 \tilde{B}} + \frac{\frac{\mathbf{q} \tilde{A} \left( \tilde{D}_A - \tilde{D}_B \right)}{\tilde{B}} + \frac{\mathbf{p} \tilde{\alpha} \left( \tilde{D}_B - \tilde{D}_\alpha \right)}{\lambda \tilde{B}}}{r} + \tilde{\alpha} \left( -\frac{\partial_r \frac{\mathbf{p}}{r}}{\lambda^3 \tilde{B}} + \frac{\tilde{A} \left( -\partial_r \tilde{K} + \partial_r \tilde{K}_\Delta + 3 \tilde{D}_B \tilde{K}_\Delta \right)}{3 \tilde{B}} \right)$$

## The evolution equation for the perfect fluid / dust

EoM\$mEvol // dump

$$\partial_t \hat{D} = \partial_r \hat{D} \beta + \partial_r \beta \hat{D} + \frac{-2 v^r \alpha \hat{D} + 2 \beta \hat{D}}{r} + \alpha \left( -\partial_r \hat{D} v^r - \partial_r v^r \hat{D} - v^r \hat{D} D_\alpha \right)$$

$$\partial_t \hat{S}_r = \partial_r \hat{S}_r \beta + 2 \partial_r \beta \hat{S}_r + \frac{-2 v^r \alpha \hat{S}_r + 2 \beta \hat{S}_r}{r} + \alpha \left( -\partial_r \hat{S}_r v^r - \partial_r v^r \hat{S}_r + v^r D_A \hat{S}_r - D_\alpha \left( \hat{D} + \hat{\tau} + v^r \hat{S}_r \right) \right)$$

$$\partial_t \hat{\tau} = \partial_r \hat{\tau} \beta + \partial_r \beta \hat{\tau} + \frac{-2 v^r \alpha \hat{\tau} + 2 \beta \hat{\tau}}{r} + \alpha \left( -\partial_r \hat{\tau} v^r - \partial_r v^r \hat{\tau} - v^r \hat{\tau} D_\alpha - \frac{D_\alpha \hat{S}_r}{A^2} + v^r K_1 \hat{S}_r \right)$$

$$v^r = \frac{\hat{S}_r}{A^2 \left( \epsilon R + \hat{D} + \hat{\tau} \right)}$$

$$\partial_r v^r = \frac{\partial_r \hat{S}_r \left( \hat{D} + \hat{\tau} \right) - \left( \partial_r \hat{D} + \partial_r \hat{\tau} \right) \hat{S}_r - 2 \left( \hat{D} + \hat{\tau} \right) D_A \hat{S}_r}{A^2 \left( \epsilon R + \hat{D} + \hat{\tau} \right)^2}$$

$$\text{pf}\rho = \frac{\hat{D} + \hat{\tau}}{A B^2}$$

$$\text{pf}j = \frac{\hat{S}_r}{A B^2}$$

$$\text{pf}J_1 = \frac{v^r \hat{S}_r}{A B^2}$$

$$\text{pf}J_2 = 0$$

## The constraint equations (without sources)

EoM\$constr1 // dump

$$\begin{aligned}
 C_{g,sc} &= \frac{\frac{\sigma}{A B} + \frac{\sigma+2 D_A-6 D_B}{A^2}}{r} + \frac{-2 \partial_r D_B + 2 D_A D_B - 3 D_B^2}{A^2} + \frac{1}{3} (K^2 - K_\Delta^2) \\
 C_{f,sc} &= \frac{\frac{\tilde{\sigma}}{\tilde{A} \tilde{B}} + \frac{\tilde{\sigma}+2 \tilde{D}_A-6 \tilde{D}_B}{\tilde{A}^2}}{r} + \frac{-2 \partial_r \tilde{D}_B + 2 \tilde{D}_A \tilde{D}_B - 3 \tilde{D}_B^2}{\tilde{A}^2} + \frac{1}{3} (\tilde{K}^2 - \tilde{K}_\Delta^2) \\
 C_{g,vec} &= \frac{2 K_\Delta}{r} + \frac{2}{3} (-\partial_r K + \partial_r K_\Delta + 3 D_B K_\Delta) \\
 C_{f,vec} &= \frac{2 \tilde{K}_\Delta}{r} + \frac{2}{3} (-\partial_r \tilde{K} + \partial_r \tilde{K}_\Delta + 3 \tilde{D}_B \tilde{K}_\Delta) \\
 C_{bim} &= \frac{\partial_r p \langle R \rangle_1^2}{\lambda} + \frac{p \left( \frac{2 \langle R \rangle_1 A R}{\tilde{A}} + \frac{2 \langle R \rangle_1 \tilde{A}}{A} \right)}{r} + \\
 &\quad p \left( \frac{2 \langle R \rangle_2 \tilde{A} D_B}{A} + \frac{2 \langle R \rangle_1 A R \tilde{D}_B}{\tilde{A}} \right) + \frac{1}{3} \tilde{A} \left( (-2 \langle R \rangle_1 + 3 \langle R \rangle_1^2) \tilde{K} + 2 \left( \langle R \rangle_2 \lambda (-K + K_\Delta) + \langle R \rangle_1 \tilde{K}_\Delta \right) \right) + \\
 &\quad A \left( -\frac{1}{3} \langle R \rangle_1^2 (K + 2 K_\Delta) - \frac{2}{3} \langle R \rangle_1 (K - K_\Delta + R \lambda (-\tilde{K} + \tilde{K}_\Delta)) \right)
 \end{aligned}$$

## The g-sources

EoM\$sources[[ ; ; 4]] // dump

$$\begin{aligned}
 g_\rho &= -\langle R \rangle_0^2 + \frac{\hat{D} + \hat{t}}{A B^2} - \frac{\langle R \rangle_1^2 \lambda \tilde{A}}{A} \\
 g_j &= -\langle R \rangle_1^2 p \tilde{A} + \frac{\hat{S}_r}{A B^2} \\
 g_{JK_1} &= -\langle R \rangle_0^1 - \frac{\langle R \rangle_1^2 p^2 \tilde{A}}{A \lambda} + \frac{\left( \frac{-2 \langle R \rangle_1 + \langle R \rangle_1^2}{2 \lambda} - \frac{\langle R \rangle_1 \tilde{A}}{A} \right) \tilde{\alpha}}{\alpha} + \frac{-\frac{(2 \langle R \rangle_1 + \langle R \rangle_1^2) \tilde{A}}{2 \lambda} + \frac{\hat{D} + \hat{t} + v^r \hat{S}_r}{2 B^2}}{A} \\
 g_{JK_2} &= -\frac{\langle R \rangle_0^2 (\hat{D} + \hat{t} - v^r \hat{S}_r)}{2 A B^2} - \frac{\langle R \rangle_1^2 \tilde{A} (\hat{D} + \hat{t} - v^r \hat{S}_r)}{4 A^2 B^2 \lambda} - \frac{\langle R \rangle_1^2 \tilde{\alpha} (\hat{D} + \hat{t} - v^r \hat{S}_r)}{4 A B^2 \alpha \lambda}
 \end{aligned}$$

## The f-sources

EoM\$sources[[- 4 ; ;]] // dump

$$\begin{aligned}
 f_{JK} &= -\frac{\langle R \rangle_1^2 p^2 \alpha \tilde{A}}{A \lambda} + \alpha \left( -\langle R \rangle_0^1 - 2 \langle R \rangle_0^2 - \frac{(2 \langle R \rangle_1 + 3 \langle R \rangle_1^2) \tilde{A}}{2 A \lambda} \right) + \left( -\frac{2 \langle R \rangle_1 + \langle R \rangle_1^2}{2 \lambda} - \frac{\langle R \rangle_2 \tilde{A}}{A} \right) \tilde{\alpha} + \frac{\alpha (3 \hat{D} + 3 \hat{t} - v^r \hat{S}_r)}{2 A B^2} \\
 f_{JK_\Delta} &= \langle R \rangle_2^1 \left( \frac{R}{\lambda} - \frac{\tilde{A}}{A} \right) \tilde{\alpha} + \alpha \left( -\frac{\langle R \rangle_1^2 p^2 \tilde{A}}{A \lambda} + \langle R \rangle_1^1 \left( R - \frac{\tilde{A}}{A \lambda} \right) + \frac{v^r \hat{S}_r}{A B^2} \right) \\
 f_{JK} &= \alpha \left( -\frac{\langle R \rangle_1^2 + 2 \langle R \rangle_2^1 R}{2 R^2 \lambda} - \frac{\langle R \rangle_1^1 A}{R \tilde{A}} \right) + \left( -\frac{2 \langle R \rangle_2^2 + \langle R \rangle_3^1 R}{R^2} - \frac{A (3 \langle R \rangle_1^2 + 2 \langle R \rangle_2^1 R)}{2 R^2 \lambda \tilde{A}} \right) \tilde{\alpha} - \frac{\langle R \rangle_1^2 A p^2 \tilde{\alpha}}{R^2 \lambda \tilde{A}} \\
 f_{JK_\Delta} &= \frac{\langle R \rangle_1^1 \alpha \left( \frac{1}{\lambda} - \frac{A R}{\tilde{A}} \right)}{R^2} + \left( \frac{\langle R \rangle_2^1 \left( 1 - \frac{A R}{\lambda \tilde{A}} \right)}{R^2} - \frac{\langle R \rangle_1^2 A p^2}{R^2 \lambda \tilde{A}} \right) \tilde{\alpha}
 \end{aligned}$$

## The constraint equations

EoM\$constr2 // dump

$$\begin{aligned}
 C_1 &= \frac{\frac{\sigma}{A B} + \frac{\sigma+2 D_A-6 D_B}{A^2}}{r} + \frac{-2 \partial_r D_B + 2 D_A D_B - 3 D_B^2}{A^2} + \frac{1}{3} (K^2 - K_\Delta^2) - \boxed{g\rho} \kappa_g \\
 C_2 &= -\boxed{f\rho} \kappa_f + \frac{\frac{\tilde{\sigma}}{\tilde{A} \tilde{B}} + \frac{\tilde{\sigma}+2 \tilde{D}_A-6 \tilde{D}_B}{\tilde{A}^2}}{r} + \frac{-2 \partial_r \tilde{D}_B + 2 \tilde{D}_A \tilde{D}_B - 3 \tilde{D}_B^2}{\tilde{A}^2} + \frac{1}{3} (\tilde{K}^2 - \tilde{K}_\Delta^2) \\
 C_3 &= \kappa_f \left( \frac{1}{3} A (-\partial_r K + \partial_r K_\Delta + 3 D_B K_\Delta) - \frac{\kappa_g \hat{S}_r}{2 B^2} \right) + \frac{A K_\Delta \kappa_f + R^2 \tilde{A} \kappa_g \tilde{K}_\Delta}{r} + \frac{1}{3} R^2 \tilde{A} \kappa_g (-\partial_r \tilde{K} + \partial_r \tilde{K}_\Delta + 3 \tilde{D}_B \tilde{K}_\Delta) \\
 C_4 &= \frac{\partial_r p \langle R \rangle_1^2}{\lambda} + \frac{p \left( \frac{2 \langle R \rangle_1^1 A R}{\tilde{A}} + \frac{2 \langle R \rangle_1^1 \tilde{A}}{A} \right)}{r} + \\
 &\quad p \left( \frac{2 \langle R \rangle_2^1 \tilde{A} D_B}{A} + \frac{2 \langle R \rangle_1^1 A R \tilde{D}_B}{\tilde{A}} \right) + \frac{1}{3} \tilde{A} \left( (-2 \langle R \rangle_1^1 + 3 \langle R \rangle_1^2) \tilde{K} + 2 \left( \langle R \rangle_2^1 \lambda (-K + K_\Delta) + \langle R \rangle_1^1 \tilde{K}_\Delta \right) \right) + \\
 &\quad A \left( -\frac{1}{3} \langle R \rangle_1^2 (K + 2 K_\Delta) - \frac{2}{3} \langle R \rangle_1^1 (K - K_\Delta + R \lambda (-\tilde{K} + \tilde{K}_\Delta)) \right)
 \end{aligned}$$

## The p-equations

EoM\$pEq\$ // dump

$$\begin{aligned}
 p_g &= -\frac{2 K_\Delta}{r \langle R \rangle_1^2 \tilde{A} \kappa_g} - \frac{2 (-\partial_r K + \partial_r K_\Delta + 3 D_B K_\Delta)}{3 \langle R \rangle_1^2 \tilde{A} \kappa_g} + \frac{\hat{S}_r}{\langle R \rangle_1^2 A B^2 \tilde{A}} \\
 p_f &= \frac{2 \tilde{B}^2 \tilde{K}_\Delta}{r \langle R \rangle_1^2 A B^2 \kappa_f} + \frac{2 \tilde{B}^2 (-\partial_r \tilde{K} + \partial_r \tilde{K}_\Delta + 3 \tilde{D}_B \tilde{K}_\Delta)}{3 \langle R \rangle_1^2 A B^2 \kappa_f} \\
 \partial_t p &= \partial_r p q + \frac{p^2 \left( -\frac{2 \langle R \rangle_1^1 \alpha \tilde{B}}{\langle R \rangle_1^2 A (1+\lambda) \tilde{A}} + \frac{2 \langle R \rangle_1^1 \tilde{B} \tilde{\alpha}}{\langle R \rangle_1^2 A (1+\lambda) \tilde{A}} \right)}{r} + \\
 &\quad \alpha \left( \frac{\frac{2 \langle R \rangle_1^1 \tilde{B} (\sigma - \lambda \tilde{\sigma})}{\langle R \rangle_1^2 \tilde{A}} + \lambda \left( -\frac{2 \langle R \rangle_1^1 D_B}{\langle R \rangle_1^2} - D_\alpha \right)}{A} + \frac{2 \langle R \rangle_1^1 R \tilde{D}_B}{\langle R \rangle_1^2 \tilde{A}} \right) + \tilde{\alpha} \left( \frac{-\frac{2 \langle R \rangle_1^1 \tilde{B} (-\lambda \sigma + \tilde{\sigma})}{\langle R \rangle_1^2 \tilde{A}} - \frac{2 \langle R \rangle_1^1 D_B}{\langle R \rangle_1^2}}{A} + \frac{\lambda \left( \frac{2 \langle R \rangle_1^1 R \tilde{D}_B}{\langle R \rangle_1^2} + \tilde{D}_\alpha \right)}{\tilde{A}} \right) + \\
 &\quad p \left( \frac{1}{3} \alpha \left( K + \frac{2 \langle R \rangle_1^1 (K - K_\Delta)}{\langle R \rangle_1^2} + 2 K_\Delta \right) + \frac{\tilde{\alpha} \left( (-2 \langle R \rangle_1^1 + 3 \langle R \rangle_1^2) \tilde{K} + 2 \langle R \rangle_1^1 \tilde{K}_\Delta \right)}{3 \langle R \rangle_1^2} \right)
 \end{aligned}$$

## The shifts

**EoM\$shifts // dump**

$$\beta = q + \frac{p \alpha}{A \lambda}$$

$$\tilde{\beta} = q - \frac{p \tilde{\alpha}}{\lambda \tilde{A}}$$

$$\partial_r \beta = \partial_r q + \frac{\partial_r p \alpha}{A \lambda^3} + \frac{p \alpha (-D_A + D_\alpha)}{A \lambda}$$

$$\partial_r \tilde{\beta} = \partial_r q - \frac{\partial_r p \tilde{\alpha}}{\lambda^3 \tilde{A}} + \frac{p \tilde{\alpha} (\tilde{D}_A - \tilde{D}_\alpha)}{\lambda \tilde{A}}$$

$$\partial_r \frac{\beta}{r} = \partial_r \frac{q}{r} + \frac{\partial_r \frac{p}{r} \alpha}{A \lambda^3} - \frac{p^3 \alpha}{r^2 A \lambda^3} + \frac{p \alpha (-D_A + D_\alpha)}{r A \lambda}$$

$$\partial_r \frac{\tilde{\beta}}{r} = \partial_r \frac{q}{r} - \frac{\partial_r \frac{p}{r} \tilde{\alpha}}{\lambda^3 \tilde{A}} + \frac{p^3 \tilde{\alpha}}{r^2 \lambda^3 \tilde{A}} + \frac{p \tilde{\alpha} (\tilde{D}_A - \tilde{D}_\alpha)}{r \lambda \tilde{A}}$$

## The lapse ratio

**EoM\$lapseRatios[[3 ;; 3]] // dump**

$$W_c = -r^2 A^2 B^2 (1 + p^2) R^2 \lambda \tilde{A}^2 (\beta_1 + R (2 \beta_2 + R \beta_3))$$

**EoM\$lapseRatios[[1 ;; 1]] // dump**

$$\begin{aligned} W_g = & \frac{2}{3} r A B^2 p R^2 \lambda \tilde{A} \left( 2 A^2 p^2 R (K - K_\Delta) \tilde{D}_B (\beta_1 + R \beta_2)^2 + \right. \\ & A^2 R (K - K_\Delta) \tilde{D}_B \left( 2 (\beta_1 + R \beta_2)^2 + \lambda^2 (\beta_1^2 + 2 R^2 \beta_2^2 + R \beta_1 (2 \beta_2 - R \beta_3)) \right) + A R \lambda \tilde{A} \\ & \left( -\lambda D_B (\tilde{K} - \tilde{K}_\Delta) (3 \beta_1^2 + 4 R^2 \beta_2^2 + R \beta_1 (6 \beta_2 - R \beta_3)) + (K - K_\Delta) \tilde{D}_B (-R \beta_2 (2 \beta_2 + 3 R \beta_3) - \beta_1 (3 \beta_2 + 4 R \beta_3)) \right) + \\ & \lambda \tilde{A}^2 D_B (R (\tilde{K} - \tilde{K}_\Delta) (-R \beta_2 (2 \beta_2 + 3 R \beta_3) - \beta_1 (3 \beta_2 + 4 R \beta_3)) + \\ & 2 \lambda (K - K_\Delta) (R \beta_2 (2 \beta_2 + 3 R \beta_3) + \beta_1 (3 \beta_2 + 4 R \beta_3)) \left. \right) + \\ & R \lambda^2 \left( A^2 B^2 R^2 \tilde{D}_B^2 \left( 4 A R \lambda (\beta_1 + R \beta_2)^2 - \tilde{A} (\beta_1^2 + 5 R \beta_1 (\beta_2 + R \beta_3) + R^2 \beta_2 (2 \beta_2 + 3 R \beta_3)) \right) - \right. \\ & 2 A B^2 R^2 \lambda \tilde{A} D_B \tilde{D}_B \left( A \lambda (3 \beta_1^2 + 4 R^2 \beta_2^2 + R \beta_1 (6 \beta_2 - R \beta_3)) + \tilde{A} (-R \beta_2 (2 \beta_2 + 3 R \beta_3) - \beta_1 (3 \beta_2 + 4 R \beta_3)) \right) + \\ & \tilde{A}^2 \left( -A B^2 R \lambda D_B^2 (-3 \beta_1^2 - 6 R \beta_1 \beta_2 - 4 R^2 \beta_2^2 + 2 R^2 (\beta_1 + R \beta_2) \beta_3 + R^4 \beta_3^2) + \right. \\ & A^2 \tilde{A} (\beta_1 - R^2 \beta_3) (\beta_1 + R (2 \beta_2 + R \beta_3)) + A^3 R \lambda (-\beta_1 + R^2 \beta_3) (\beta_1 + R (2 \beta_2 + R \beta_3)) + B^2 R \tilde{A} D_B^2 \\ & \left. (p^2 (-\beta_2 (3 \beta_1 + 2 R \beta_2) - 5 R (\beta_1 + R \beta_2) \beta_3 - R^3 \beta_3^2) + \lambda^2 (\beta_2 + R \beta_3) (-3 \beta_1 + R (-2 \beta_2 + R \beta_3))) \right) + \\ & r^2 \left( \frac{1}{2} R^2 \lambda^2 \tilde{A}^2 \kappa_g (\beta_1 + R (2 \beta_2 + R \beta_3)) \left( 4 p \lambda \tilde{A} \hat{S}_r (\beta_2 + R \beta_3) - 2 A \tilde{A} (p^2 (\hat{D} + \hat{e}) + v^r \lambda^2 \hat{S}_r) (\beta_2 + R \beta_3) + \right. \right. \\ & 2 A^3 B^2 \lambda (\beta_1 + R \beta_2) (2 \beta_0 + 3 R \beta_1 - R^3 \beta_3) + A^2 \left( \lambda (\hat{D} + \hat{e} - v^r \hat{S}_r) (\beta_1 - R^2 \beta_3) + \right. \\ & B^2 \tilde{A} (3 \beta_1^2 + 2 \beta_2 (\beta_0 + 3 R^2 \beta_2) + 2 R (\beta_0 + R^2 \beta_2) \beta_3 - R^4 \beta_3^2 + 6 R \beta_1 (2 \beta_2 + R \beta_3)) \left. \right) + \\ & \frac{1}{9} A^2 B^2 R^2 \lambda^2 \tilde{A}^2 \left( -p^2 \tilde{A} (K - K_\Delta)^2 (\beta_2 + R \beta_3) (3 \beta_1 + R (2 \beta_2 - R \beta_3)) + \right. \\ & A \lambda \left( -4 R^2 (\tilde{K} - \tilde{K}_\Delta)^2 (\beta_1 + R \beta_2)^2 + (K - K_\Delta)^2 (-3 \beta_1^2 - 6 R \beta_1 \beta_2 - 4 R^2 \beta_2^2 + 2 R^2 (\beta_1 + R \beta_2) \beta_3 + R^4 \beta_3^2) + \right. \\ & 2 R \lambda (K - K_\Delta) (\tilde{K} - \tilde{K}_\Delta) (3 \beta_1^2 + 4 R^2 \beta_2^2 + R \beta_1 (6 \beta_2 - R \beta_3)) \left. \right) + \\ & \tilde{A} \left( \lambda^2 (K - K_\Delta)^2 (-\beta_2 (3 \beta_1 + 2 R \beta_2) - 5 R (\beta_1 + R \beta_2) \beta_3 - R^3 \beta_3^2) + R (\tilde{K} - \tilde{K}_\Delta)^2 (\beta_1 + R \beta_2) \right. \\ & \left. (\beta_1 - R (2 \beta_2 + 3 R \beta_3)) + 2 R \lambda (K - K_\Delta) (\tilde{K} - \tilde{K}_\Delta) (R \beta_2 (2 \beta_2 + 3 R \beta_3) + \beta_1 (3 \beta_2 + 4 R \beta_3)) \left. \right) \right) - \\ & \frac{1}{2} A^2 B^2 \lambda^2 \tilde{A}^2 \kappa_f (\beta_1 + R (2 \beta_2 + R \beta_3)) \left( 6 A R \lambda (\beta_1 + R \beta_2) (\beta_1 + R (2 \beta_2 + R \beta_3)) + \right. \\ & \left. \tilde{A} (-\beta_1^2 + 2 R \beta_1 (\beta_2 + R (3 \beta_3 + R \beta_4)) + R^2 (6 \beta_2^2 + 3 R^2 \beta_3^2 + 2 R \beta_2 (6 \beta_3 + R \beta_4))) \right) \end{aligned}$$

EoM\$lapseRatios[[2 ;; 2]] // dump

$$\begin{aligned}
W_f = & \frac{2}{3} r A B^2 p R^2 \lambda \tilde{A} \left( 2 p^2 \tilde{A}^2 D_B \left( -\tilde{K} + \tilde{K}_\Delta \right) (\beta_2 + R \beta_3) (\beta_1 + R (2 \beta_2 + R \beta_3)) + \right. \\
& \tilde{A}^2 D_B (\tilde{K} - \tilde{K}_\Delta) (\lambda^2 (2 \beta_2 (\beta_1 + 4 R \beta_2) + R (\beta_1 + 12 R \beta_2) \beta_3 + 5 R^3 \beta_3^2) - 2 (\beta_2 + R \beta_3) (\beta_1 + R (2 \beta_2 + R \beta_3))) + \\
& A^2 R \lambda \tilde{D}_B \left( (K - K_\Delta) (-R \beta_2 (2 \beta_2 + 3 R \beta_3) - \beta_1 (3 \beta_2 + 4 R \beta_3)) + \right. \\
& 2 R \lambda (\tilde{K} - \tilde{K}_\Delta) (R \beta_2 (2 \beta_2 + 3 R \beta_3) + \beta_1 (3 \beta_2 + 4 R \beta_3)) \left. \right) + A R \lambda \tilde{A} \left( D_B (\tilde{K} - \tilde{K}_\Delta) \right. \\
& \left. (-R \beta_2 (2 \beta_2 + 3 R \beta_3) - \beta_1 (3 \beta_2 + 4 R \beta_3)) + \lambda (K - K_\Delta) \tilde{D}_B (-4 \beta_2^2 - 6 R \beta_2 \beta_3 + \beta_3 (\beta_1 - 3 R^2 \beta_3)) \right) \left. \right) + \\
\lambda^2 \left( \lambda \tilde{A}^3 \left( -4 B^2 R^2 D_B^2 (\beta_2 + R \beta_3)^2 + A^2 (-\beta_1 + R^2 \beta_3) (\beta_1 + R (2 \beta_2 + R \beta_3)) \right) + \right. \\
& A^3 B^2 R^3 \tilde{D}_B^2 (\lambda^2 (\beta_1 + R \beta_2) (-\beta_1 + R (2 \beta_2 + 3 R \beta_3)) + p^2 (\beta_1^2 + 5 R \beta_1 (\beta_2 + R \beta_3) + R^2 \beta_2 (2 \beta_2 + 3 R \beta_3))) - \\
& A^2 B^2 R^2 \lambda \tilde{A} \tilde{D}_B \left( 4 R (\beta_2 + R \beta_3) \left( D_B (\beta_1 + R \beta_2) + R (-D_B + \tilde{D}_B) (\beta_2 + R \beta_3) \right) + \right. \\
& (\beta_1 + R (2 \beta_2 + R \beta_3)) \left( 2 R D_B (\beta_2 + 2 R \beta_3) - \tilde{D}_B (\beta_1 + R^2 \beta_3) \right) \left. \right) + \\
& A R \tilde{A}^2 \left( A^2 ((-p^2 + \lambda^2) (\beta_1 + R \beta_2) - R (\beta_2 + R \beta_3)) (\beta_1 + R (2 \beta_2 + R \beta_3)) + \right. \\
& B^2 R D_B (-4 R (D_B - 2 \lambda^2 \tilde{D}_B) (\beta_2 + R \beta_3)^2 + (2 R (D_B - \lambda^2 \tilde{D}_B) \beta_3 + 3 D_B (\beta_2 + R \beta_3)) (\beta_1 + R (2 \beta_2 + R \beta_3))) \left. \right) \left. \right) + \\
r^2 \left( \frac{1}{2} A^2 R^2 \lambda^2 \tilde{A}^2 \kappa_g (\beta_1 + R (2 \beta_2 + R \beta_3)) \left( A B^2 (3 \beta_1^2 + 2 \beta_2 (\beta_0 + 3 R^2 \beta_2) + 2 R (\beta_0 + R^2 \beta_2) \beta_3 - \right. \right. \\
& R^4 \beta_3^2 + 6 R \beta_1 (2 \beta_2 + R \beta_3)) + 2 (\beta_2 + R \beta_3) \left( \hat{D} + \hat{e} + 3 B^2 \lambda \tilde{A} (\beta_1 + R (2 \beta_2 + R \beta_3)) \right) \left. \right) + \\
\frac{1}{9} A^2 B^2 R^2 \lambda^2 \tilde{A}^2 \left( -A p^2 R (\tilde{K} - \tilde{K}_\Delta)^2 (\beta_1 + R \beta_2) (\beta_1 - R (2 \beta_2 + 3 R \beta_3)) + \right. \\
& A \left( (K - K_\Delta)^2 (\beta_2 + R \beta_3) (3 \beta_1 + R (2 \beta_2 - R \beta_3)) + R \lambda^2 (\tilde{K} - \tilde{K}_\Delta)^2 (\beta_1^2 + 5 R \beta_1 (\beta_2 + R \beta_3) + \right. \\
& R^2 \beta_2 (2 \beta_2 + 3 R \beta_3)) + 2 R \lambda (K - K_\Delta) (\tilde{K} - \tilde{K}_\Delta) (-R \beta_2 (2 \beta_2 + 3 R \beta_3) - \beta_1 (3 \beta_2 + 4 R \beta_3)) \left. \right) + \\
& \lambda \tilde{A} \left( 4 (K - K_\Delta)^2 (\beta_2 + R \beta_3)^2 + 2 R \lambda (K - K_\Delta) (\tilde{K} - \tilde{K}_\Delta) (-4 \beta_2^2 - 6 R \beta_2 \beta_3 + \beta_3 (\beta_1 - 3 R^2 \beta_3)) + \right. \\
& (\tilde{K} - \tilde{K}_\Delta)^2 (-\beta_1^2 - 2 R \beta_1 (\beta_2 + R \beta_3) + R^2 (4 \beta_2^2 + 6 R \beta_2 \beta_3 + 3 R^2 \beta_3^2)) \left. \right) \left. \right) - \\
\frac{1}{2} A^2 B^2 \lambda^2 \tilde{A}^2 \kappa_f (\beta_1 + R (2 \beta_2 + R \beta_3)) \left( 2 \lambda \tilde{A} (\beta_2 + R \beta_3) (-\beta_1 + R^2 (3 \beta_3 + 2 R \beta_4)) + \right. \\
& A (-\beta_1 + R (2 \beta_2 + R \beta_3)) (\beta_1 - R (2 \beta_2 + 3 R \beta_3)) - \\
& \left. \left. 2 p^2 R (\beta_1 + R \beta_2) (\beta_2 + R (2 \beta_3 + R \beta_4)) + 2 R \lambda^2 (\beta_1 + R \beta_2) (\beta_2 + R (2 \beta_3 + R \beta_4)) \right) \right) \left. \right)
\end{aligned}$$
